# Supplementary material for: Physics-informed dynamic mode decomposition (piDMD)
Source: arXiv:2112.04307 source file (2021-12-08)
Supplement: Supplementary file 1 [file supplement.tex]

\subsubsection{Details of calculation of variance for self-adjoint DMD problem}
\textcolor{red}{Put in supplementary material.}
The entries of $\bC$ in \eqref{Eq:symL} are given by
\begin{align}
	\tilde{\bC}_{i,j} = \sum^{n}_{l=1} \sum^{n}_{k=1} 
	\epsilon_{k,l} \bU_{k,i} \bV_{l,j}
\end{align}
The entries of $\tilde{\bL}$ are
\begin{align}
	\tilde{\bL}_{i,j} = \tilde{\bL}_{j,i} = 
	\sum^{n}_{l=1} \sum^{n}_{k=1} 
	\epsilon_{k,l} \frac{\sigma_i {\bU_{k,j} \bV_{l,i}} + \sigma_j \bU_{k,i} \bV_{l,j}}{\sigma_i^2 + \sigma_j^2}
\end{align}
Let's assume that the data are real, so we don't need to use complex conjugates
We first compute the covariance of the entries of $\bL$:
\begin{align*}
	&\Cov\left[ \bL_{i,j},\bL_{r,s} \right]
	= \E \left[ \bL_{i,j}{\bL_{r,s}} \right]\\
	&=\left( \sigma_i^2 + \sigma_j^2 \right)^{-1}  
	 \left( \sigma_r^2 + \sigma_s^2 \right)^{-1}  \sum^{n}_{l=1} \sum^{n}_{k=1} \sum^{n}_{p=1} \sum^{n}_{q=1} 
	\epsilon_{k,l} \epsilon_{p,q}\left( {\sigma_i {\bU_{k,j} \bV_{l,i}} + \sigma_j \bU_{k,i} \bV_{l,j}}\right)
	\left(\sigma_i {\bU_{q,s} \bV_{p,r}} + \sigma_j {\bU_{q,r} \bV_{p,s}}\right)\\
	&=\left( \sigma_i^2 + \sigma_j^2 \right)^{-1}  
	 \left( \sigma_r^2 + \sigma_s^2 \right)^{-1}	
	 \sum^{n}_{l=1} \sum^{n}_{k=1} \E{\varsigma_{k,l}^2}
	\left( {\sigma_i {\bU_{k,j} \bV_{l,i}} + \sigma_j \bU_{k,i} \bV_{l,j}} \right)
	\left( {\sigma_r {\bU_{k,s} \bV_{l,r}} + \sigma_s {\bU_{k,r} \bV_{l,s}}} \right)\\
	& = \varsigma^2 \left( \sigma_i^2 + \sigma_j^2 \right)^{-2}  \sum^{n}_{l=1} \sum^{n}_{k=1} 
	\left( {\sigma_i {\bU_{k,j} \bV_{l,i}} + \sigma_j \bU_{k,i} \bV_{l,j}} \right)
	\left( {\sigma_r {\bU_{k,s} \bV_{l,r}} + \sigma_s {\bU_{k,r} \bV_{l,s}}} \right)\\
	& = \varsigma^2 \left( \sigma_i^2 + \sigma_j^2 \right)^{-2}  \sum^{n}_{l=1} \sum^{n}_{k=1} 
	\left( \sigma_i \sigma_r \bU_{k,j}\bU_{k,s} \bV_{l,i} \bV_{l,r} + 
			\sigma_j \sigma_r \bU_{k,i} \bU_{k,s} \bV_{l,j} \bV_{l,r} \right. \\ 
	 & \left.+	\sigma_i \sigma_s \bU_{k,j} \bU_{k,r} \bV_{l,i} \bV_{l,s}
		+	\sigma_j \sigma_s \bU_{k,i} \bU_{k,r} \bV_{l,j} \bV_{l,s} \right)\\
	& = \varsigma^2 \left( \sigma_i^2 + \sigma_j^2 \right)^{-2}  
	\left( \sigma_i^2 
		+\sigma_j^2  \right) \left(\delta_{i,s} \delta_{j,r} 
	+\delta_{i,r} \delta_{j,s} \right) \\
&=  \varsigma^2  \frac{\delta_{i,s} \delta_{j,r}+\delta_{i,r} \delta_{j,s} }{\sigma_i^2 + \sigma_j^2}.
\end{align*}
In other words
\begin{align}
	\Cov\left[ \bL_{i,j}, \, \bL_{r,s} \right] &=
\frac{\varsigma^2}{\sigma_i^2 + \sigma_j^2} \times 
	\begin{cases}
		1 & \textrm{if } i = r \neq j = s, \\
		1 & \textrm{if } i = s \neq j = r, \\
		2 & \textrm{if } i = r  = j = s, \\
		0 & \textrm{otherwise}
	\end{cases}
\end{align}
We note that
\begin{align}
	\bA_{i,j} = \sum^{n}_{k=1} \sum^{n}_{l=1} 
	\bU_{i,k} \tilde{\bL}_{k,l} \bU_{j,l}
	= \sum^{n}_{k=1} \sum^{n}_{l=1} 
	a_{k,l}
\end{align}
We use the identity
\begin{align*}
	\left( \sum^{n}_{k=1} \sum^{n}_{l=1} d_{k,l}   \right)^2
	=& \sum^{n}_{k=1} \sum^{n}_{\substack{l=1\\l\neq k}}  d_{k,l}\left( d_{k,l} + d_{l,k} \right)
	+ \sum_{k=1}^n d_{k,k}^2\\
	+& \sum_{k=1}^n \left[ \sum_{l=1}^n d_{k,l} \left( \sum_{\substack{s=1\\s \neq l}}^n d_{k,s} + \sum_{\substack{s=1 \\ s \neq k}}^n d_{s,l}   \right)
	+ \sum^{n}_{\substack{l=1\\l\neq k}}\left( 
		\sum^{n}_{\substack{s \neq l\\s\neq k}} d_{k,l} d_{l,s} 
		+\sum^{n}_{\substack{r = 1 \\r \neq l}} d_{k,r} \left( d_{l,k} +
		\sum^{n}_{\substack{s \neq l\\s\neq k}} d_{l,s} 
		\right)
\right) \right]
	% + d_{k,l} d_{l,k} + d_{k,l}\left( d_{k,k} + d_{l,l} \right)
	% + d_{k,l} \sum^{n}_{\substack{s =1\\s\neq k, \, s \neq l}} d_{s,k} + d_{s,l} + 
	% \sum^n_{r=1} d_{r,s}
\end{align*}
Thus,
\begin{align}
	&\Var(\bA_{i,j}) = \E(\bA_{i,j}^2)
	= \sum^{n}_{k=1} \sum^{n}_{l=1}  \E(a_{k,l}^2) + \E(a_{k,l} a_{l,k}) + \E(a_{k,l}\left( a_{k,k} + a_{l,l} \right))\\
	%
	%
	% &= \sum^{n}_{k=1} \sum^{n}_{l=1}  \bU_{i,k}^2 \E(\bL_{k,l}^2) \bU_{j,l}^2 
	% + \bU_{i,k} \bU_{i,l} \E(\bL_{k,l} \bL_{l,k}) \bU_{j,l}\bU_{j,k} \\
	% &+ \bU_{i,k}^2 \E(\bL_{k,l} \bL_{k,k}) \bU_{j,l} \bU_{j,k}
	% + \bU_{i,k} \bU_{i,j} \E(\bL_{k,l} \bL_{l,l}) \bU_{j,l}^2\\
	%
	%
	  &= \sum^{n}_{k=1} \sum^{n}_{\substack{l=1\\l \neq k}}  \bU_{i,k}^2 \E(\bL_{k,l}^2) \bU_{j,l}^2 
	+ \bU_{i,k} \bU_{i,l} \E(\bL_{k,l} \bL_{l,k}) \bU_{j,l}\bU_{j,k}
	+\sum_{k=1}^n \bU_{i,k}^2 \E(\bL_{k,k}^2) \bU_{j,k}^2\\
	&= \left(\sum^{n}_{k=1} \sum^{n}_{\substack{l=1\\l\neq k}}  \frac{\bU_{i,k}^2 \bU_{j,l}^2 
	+ \bU_{i,k} \bU_{i,l} \bU_{j,l}\bU_{j,k}}{\sigma_k^2 + \sigma_l^2}
	+ \sum^{n}_{k=1} \frac{\bU_{i,k}^2 \bU_{j,k}^2}{\sigma_k^2}\right)\\
	&= \sum^{n}_{k=1} \sum^{n}_{\substack{l=1}}  \frac{\bU_{i,k} \bU_{j,l}\left(\bU_{i,k} \bU_{j,l} 
	+ \bU_{i,l} \bU_{j,k}\right)}{\sigma_k^2 + \sigma_l^2}\\
	%
	% next line follows by symmetry
	&=  \sum^{n}_{k=1} \sum^{n}_{\substack{l=1}}  \frac{\left(\bU_{i,k} \bU_{j,l} 
	+ \bU_{i,l} \bU_{j,k}\right)^2}{2(\sigma_k^2 + \sigma_l^2)}
\end{align}
